# Supplementary material for: Accurate Determination of the Dynamical Polarizability of Dysprosium
Source: arXiv:1801.05658 ancillary file (2018-06-06)
Supplement: Supplementary file 1 [file PolarDy_SM.pdf]

# Supplemental material: Accurate Determination of the Dynamical Polarizability of Dysprosium

C. Ravensbergen,[1,2] V. Corre,[1,2] E. Soave,[2] M. Kreyer,[1,2] S. Tzanova,[1,2] E. Kirilov,[2] and R. Grimm[1,2]

[1] *Institut für Quantenoptik und Quanteninformation, Österreichische Akademie der Wissenschaften, 6020 Innsbruck, Austria (IQOQI)*

[2] *Institut für Experimentalphysik, Universität Innsbruck, 6020 Innsbruck, Austria*

(Dated: March 12, 2018)

In Sections I and II we present measurements on Dy testing systematic effects introduced by atomic density and temperature. Section III provides additional information on our measurement of the tensor part of the polarizability of Dy. Section IV reviews the different contributions to the uncertainty on our measurement of the polarizability of Dy.

## I. ABSENCE OF DENSITY EFFECT ON OSCILLATION FREQUENCY

Throughout our determination of the polarizability of Dy we assume that the frequency of the CoM oscillations is independent of the atomic density, as is expected in a harmonic potential. In this section we test this basic assumption by investigating the effect of density on our frequency measurements. We prepare samples of largely different atom number and determine the frequency for the same trap depth as used in the main text. The atom number is controlled through the MOT loading time. We use a standard (reduced) loading time of 4 s (0.2 s), resulting in a cloud of about $1.1 \times 10^6 (4.5 \times 10^5)$ atoms. We measure alternately using one loading time, then the other one, and repeat the procedure to eliminate the effect of possible slow drifts. After each individual measurement the temperature of the cloud is measured by ToF expansion. Based on these temperatures, the measured trap frequencies are corrected to account for the effect of anharmonicity of the trap, using the coefficient $\beta$ defined in the main text. Note, however, that we do not observe a significant correlation between temperature and atom number. The results are presented in Figure 1. A linear fit gives a slope of 0.28(70)% per million of atoms, which is consistent with the absence of a density effect. This confirms our assumption of a density independence of the oscillation frequency on the level of 1% for our standard experimental condidtions.

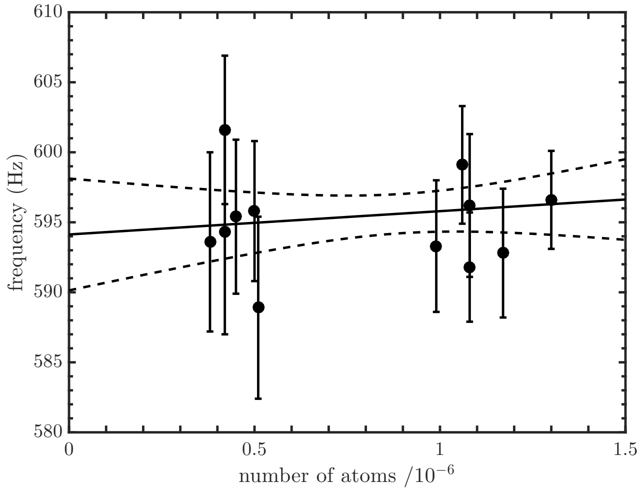


Figure 1. Test of the effect of atomic density on the oscillation frequency. The measured frequency is plotted against the atom number. The solid line is a linear fit, and the dashed line shows the 68% ($1\sigma$) confidence band.

## II. DAMPING OF OSCILLATIONS

In the main text we introduce the assumption that the damping of the CoM oscillations originates essentially from the anharmonicity of the trap: Different classes of atoms explore different regions of the trap as they oscillate, hence experiencing slightly different trap frequencies and eventually dephasing. Such a behavior would mean that the CoM oscillations that we observe result from a superposition of pure single-particle oscillations. This assumption is supported by the equal damping behavior of the two species, as pointed out in the main text, and by an estimation based on our experimental settings of the collision rate of dysprosium atoms, which yields 80 $s^{-1}$ (a similar calculation for potassium gives a collision rate of about 90 $s^{-1}$). Given the radial trap frequency of about 600 Hz (2 kHz for K), the radial motion in our trapped samples is far away from the hydrodynamic regime. Here we further test our assumption on the origin of the observed damping by considering the density and temperature dependence of the damping rate of the CoM oscillations.

From the analysis of the set of experiments presented in Sec. A we also obtain the damping rate of the oscillations. Its behavior as a function of atom number is plotted in Figure 2. A linear fit gives a slope of $+0.008(30)$ $s^{-1}$ per million atom and thus does not show any significant density dependence on the 10% level for our standard atom number. This observation support our assumption of damping being essentially due to dephasing effects.

We now turn our attention to the study of the de-

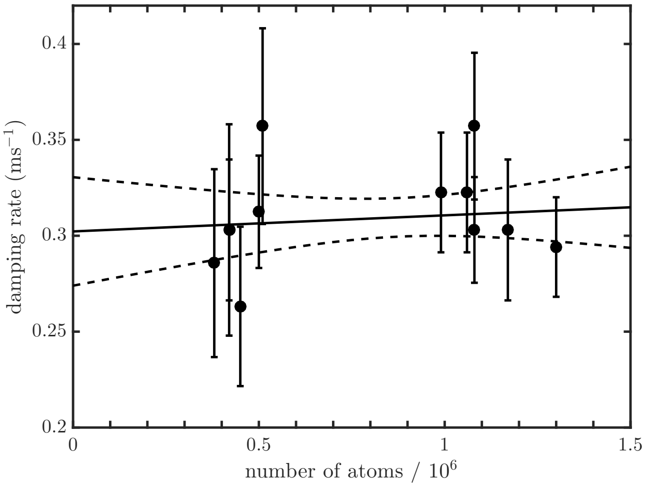


Figure 2. Density independence of the damping rate. The solid line is a linear fit, and the dashed lines show the 68% ($1\sigma$) confidence band.

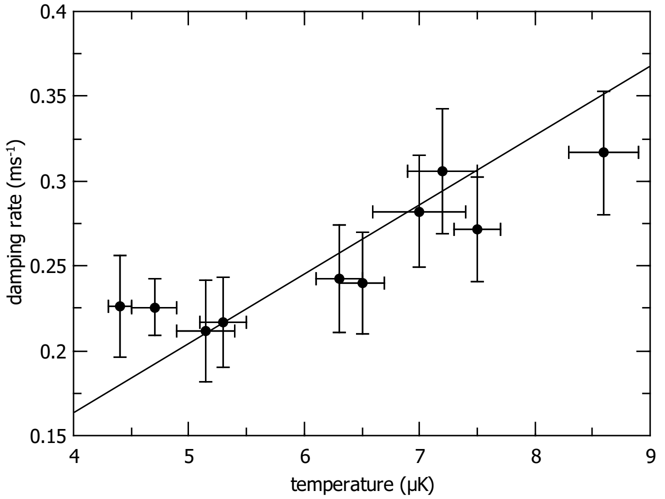


Figure 3. Temperature dependence of the damping time. The solid line is a linear fit without offset, with weights taking both horizontal and vertical error bars into account.

pendence of the damping rate on the temperature. From straightforward arguments, one expects the damping rate to be proportional to the temperature. Indeed, for small oscillation amplitudes, the anharmonic frequency shift of a particle in a Gaussian potential scales linearly with its energy, such that the width in Fourier space of the CoM oscillation increases linearly with the temperature of the cloud, finally leading to a linear dependence of the damping rate on the temperature. In the main text, we present a measurement of the dependence of the frequency on the temperature of the cloud (see Figure 3 in the main text). The analysis of the corresponding oscillation data also allows us to investigate the dependence of the damping rate of the oscillations on the temperature. The results are shown in Figure 3. We observe an increase of the damping with temperature. A linear fit without offset gives a slope of 0.409(15) $\mathrm{ms}^{-1}\mu\mathrm{K}^{-1}$, and a reduced $\chi^2$ of 0.96, showing that our simple model fits well to the data. This behavior also supports our interpretation on dephasing being the main source of damping.

## III. ERROR BUDGET OF THE FREQUENCY RATIO MEASUREMENT

We measure the trap frequency ratio in two sets of data obtained on two different days. Each set of data is corrected for the residual anharmonicity, based on the anharmonicity coefficient $\beta$ and on the measured temperatures of the two species. A part of the uncertainty originates from the statistical distribution of the measured frequency ratios $\omega_\mathrm{K}/\omega_\mathrm{Dy}$. The rest of the uncertainty originates from the error in the anharmonicity correction and has five contributions: the error on the anharmonicity coefficient $\beta$, and the error on the measured temperatures of the K and Dy clouds. The respective contributions to the absolute uncertainty on $\omega_\mathrm{K}/\omega_\mathrm{Dy}$ are listed in Table I.

Table I. Error budget for the measurement of $\omega_\mathrm{K}/\omega_\mathrm{Dy}$.

| parameter | value | uncertainty in parameter | uncertainty in frequency ratio |
|---|---|---|---|
| $T_\mathrm{Dy}$ set 1 | 8.3 $\mu$K | 0.2 $\mu$K | 0.003 |
| $T_\mathrm{K}$ set 1 | 7.6 $\mu$K | 0.3 $\mu$K | 0.004 |
| $T_\mathrm{Dy}$ set 2 | 35.7 $\mu$K | 3.2 $\mu$K | 0.015 |
| $T_\mathrm{K}$ set 2 | 30.3 $\mu$K | 2.0 $\mu$K | 0.008 |
| $\beta$ | $-4.50$ Hz/$\mu$K | 0.43 Hz/$\mu$K | 0.006 |

The total absolute uncertainty that results from the anharmonicity correction is 0.019, and the statistical uncertainty from the 10 combined individual measurements is 0.012. These two errors are quadratically combined, which finally yields the quoted uncertainty of 0.022.

## IV. MEASUREMENT OF THE TENSOR CONTRIBUTION

We measure oscillation frequencies for two different orientations of the magnetic field: Always being perpendicular to the propagation axis of the trapping laser, the field is either aligned with the polarization axis of the trapping laser, or perpendicular to it. All other parameters are kept identical. The strength of the field is in both cases 250 mG. In the latter case we take care that the spin state of the atoms adiabatically follows the rotation of the magnetic field. We measure alternately the trap frequency for one orientation of the field, then for the other one, and repeat the procedure to eliminate

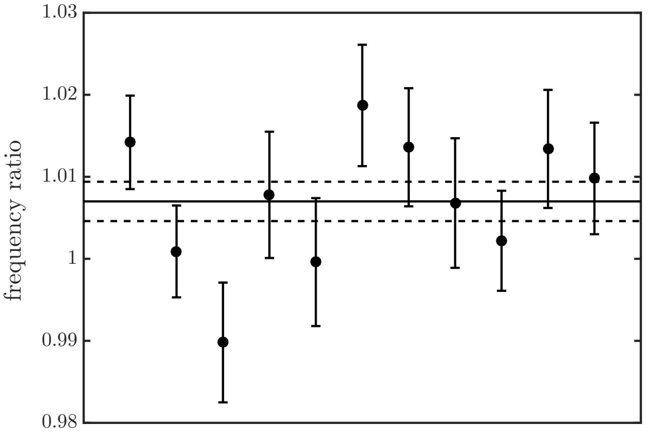


Figure 4. Repeated measurements of the frequency ratio $\omega_\parallel/\omega_\perp$. The first five points have been measured on one day, the remaining six ones on a second day. The solid line shows the weighted average$\omega_\parallel/\omega_\perp = 1.0070(20)$ with the dashed lines showing the corresponding statistical error range.

systematic effects from possible slow drifts. We measure in total 11 pairs of trap frequencies over two different days, which gives us 11 values for the frequency ratio, as shown in Figure 4. A weighted average yields $(a_s + a_t)/(a_s - a_t/2) = 1.0140(48)$.
